# Supplementary material for: Sublinear Algorithms for $(1.5+\epsilon)$-Approximate Matching
Source: arXiv:2212.00189 source file (2023-04-26)
Supplement: Supplementary file 1 [file 5-appendix_matrix_adjacency.tex]

\section{Sub-linear algorithms with adjacency matrix queries}

\label{sec:appendix:adjacency}
